# Supplementary material for: CrossLoc3D: Aerial-Ground Cross-Source 3D Place Recognition
Source: arXiv:2303.17778 source file (2023-09-29)
Supplement: Supplementary file 1 [file 3-reproduce.tex]

\section{Reproducible Results}

Due to the $100MB$ limit on the supplemental files and policy against external links, we could not provide the trained model or the \oursdata{} benchmark. Instead, we provide a simplified version of the code that can train our model from scratch on the Oxford RobotCar dataset~\cite{oxford}, and detailed instructions on installation. By following the provided instruction, we are able to reproduce similar results by choosing the best model from the first 200 epochs on a Nvidia RTX A5000 or 3090 GPU. Please refer to \textit{\textbf{training\_code.zip}}, which contains \textit{\textbf{README.md}}. In addition, we include the original training log for both Oxford RobotCar and \oursdata{} benchmark and remove any personal information in the log file. Please refer to the \textit{\textbf{log/}} folder in the root directory.

In case the environment setup is not successful, we provide another option for visualizing some query examples by one single command, which does not need as many dependencies as the training environment, and only requires some standard libraries. We save the embeddings from the output of \ours{}, so they can directly retrieved and visualized on the map within the $100MB$ file size limit. Some of the examples correspond to the visualizations in Fig.~\ref{fig:inf_vis} and Fig.~\ref{fig:failure_case}. Please refer to \textit{\textbf{visualization\_demo.zip}}, which contains \textit{\textbf{README.md}} and  \textit{\textbf{requirement.txt}}.

\begin{figure*}[t]
    \centering
    \includegraphics[width=\textwidth]{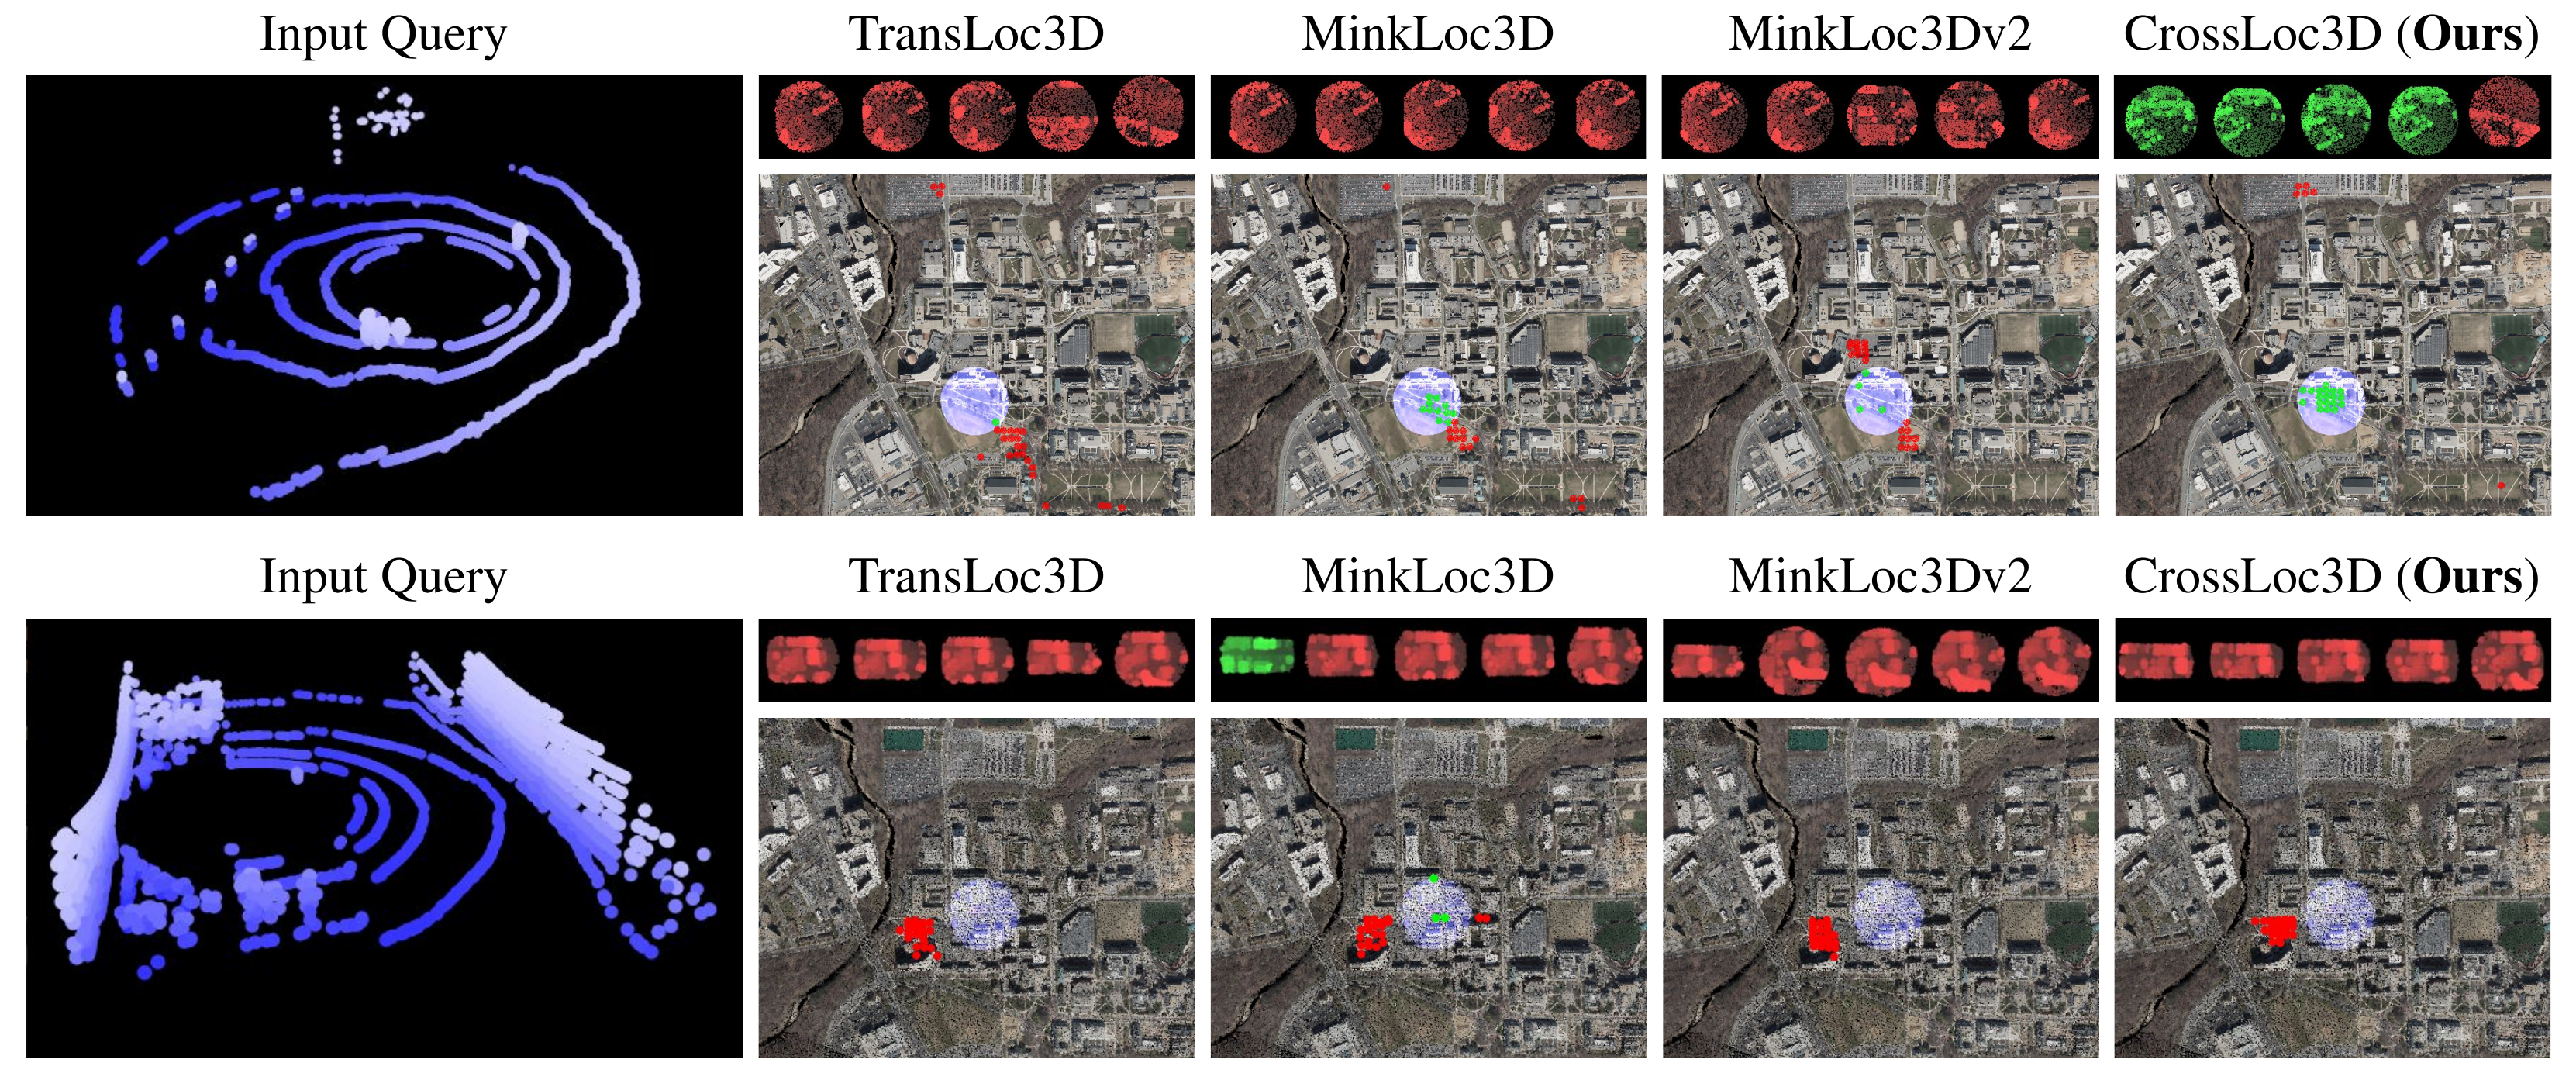}
    \caption{\textbf{Two Challenging cases for \ours{} and other SOTA methods~\cite{transloc3d, minkloc3d, minkloc3dv2}:} \textbf{For each row, left:} Input ground query (\textcolor{blue}{blue}). \textbf{For each row, top:} Top 5 retrievals (ranked from left to right) from the database of aerial data (true neighbor -- \textcolor{green}{green}, false neighbor -- \textcolor{red}{red}). \textbf{For each row, bottom:} Distributions of ground query and top 25 retrievals. 
    }
    \label{fig:failure_case}
    % \vspace{-18pt}
\end{figure*}
